# Supplementary material for: Building A Trusted Execution Environment for In-Storage Computing
Source: arXiv:2205.06361 source file (2022-05-12)
Supplement: Supplementary file 1 [file appendix.tex]

\section{Source Data of Our Experiments}
In the appendix of this paper, we present the source data of our experiments as per the request from Reviewer-A. 

\begin{figure}[!tph]
        \centering
        \includegraphics[width=1\linewidth]{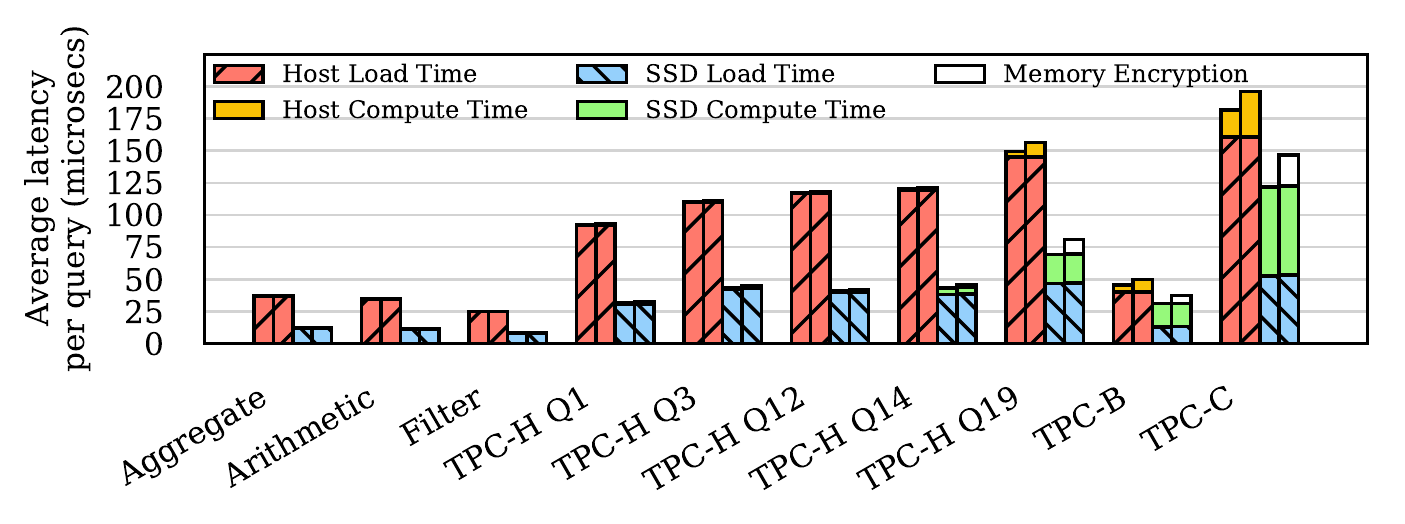}
        \vspace{-4ex}
        \caption{Performance comparison of Host, Host+SGX, ISC, and IceClave (from left to right).
        We show the performance breakdown of each scheme. This figure refers to Figure~\ref{fig:iscvsvanila} in the revised paper. }
        \label{fig:iscvsvanila-abs}
        \vspace{-3ex}
\end{figure}

\begin{figure}[!tph]
        \centering
        \includegraphics[width=\linewidth]{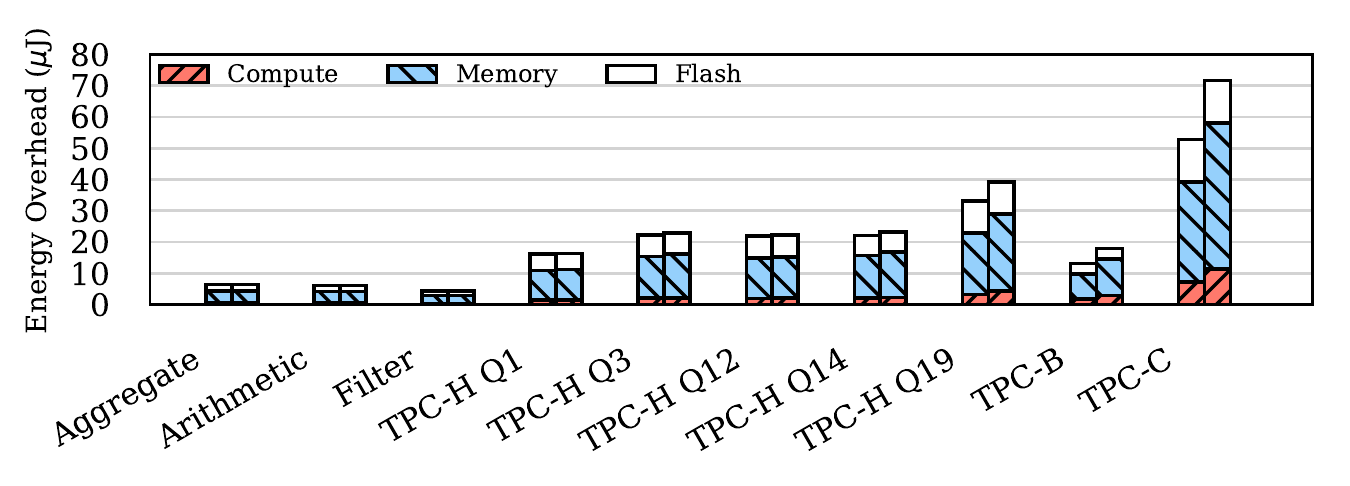}
        \vspace{-4.5ex}
        \caption{Energy overhead of IceClave. The figure refers to Figure~\ref{fig:energy} in the revised paper.}
        \label{fig:energy-abs}
        \vspace{-2ex}
\end{figure}

\begin{figure}[!tph]
        \centering
        \includegraphics[width=\linewidth]{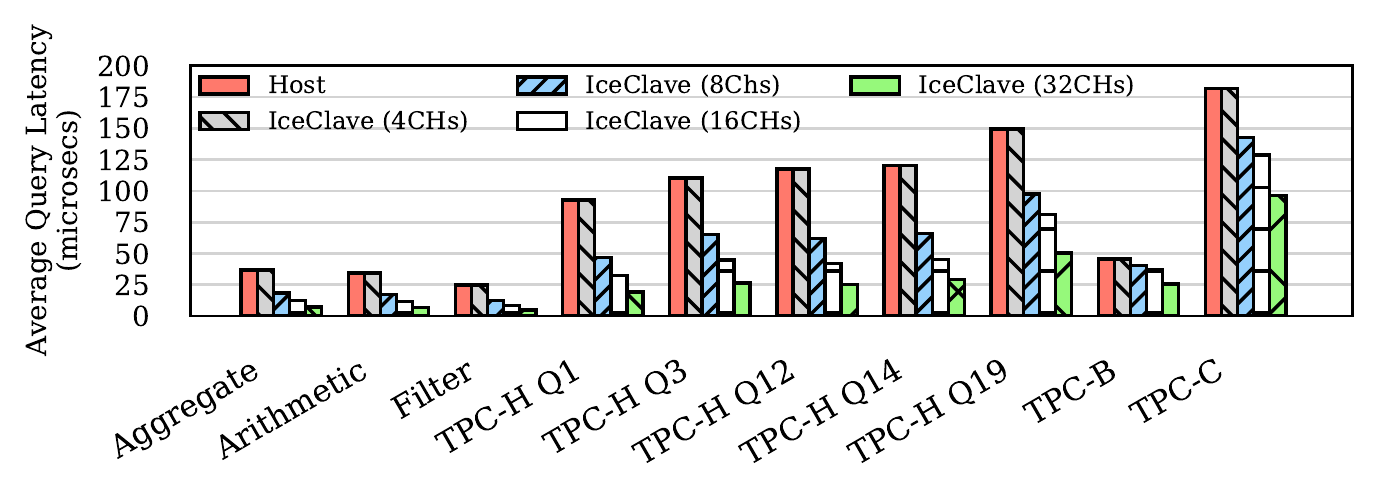}
        \vspace{-4ex}
        \caption{{IceClave performance (normalized to Host), as we vary the internal SSD bandwidth by using different number of channels. This figure refers to Figure~\ref{fig:bws} in the revised paper.}}
        \label{fig:bws-abs}
        \vspace{-4ex}
\end{figure}

\begin{figure}[!tph]
        \centering
        \includegraphics[width=\linewidth]{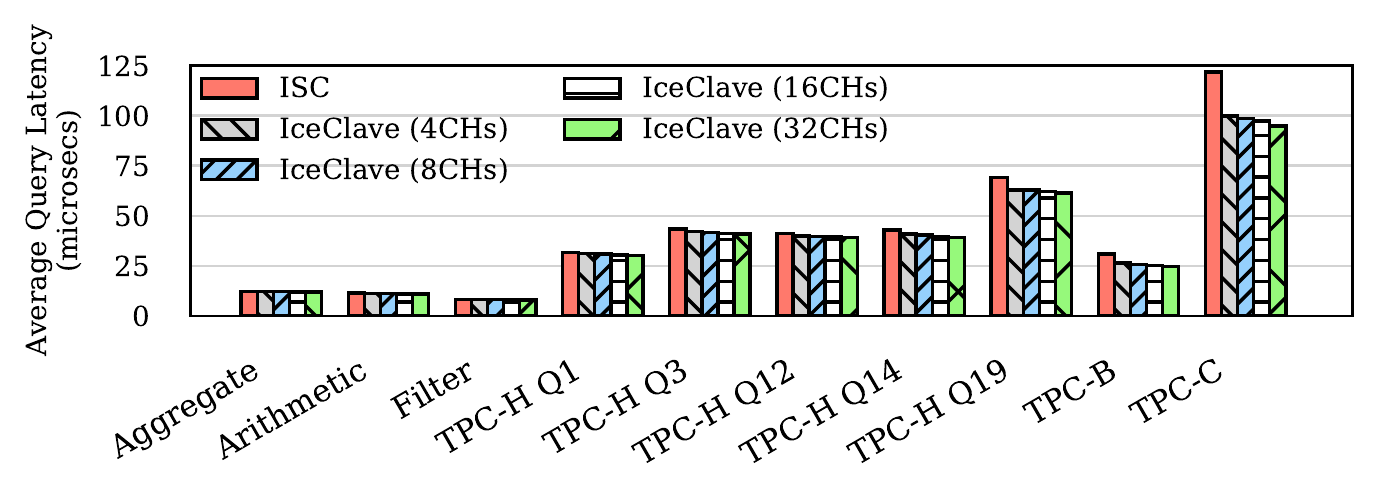}
        \vspace{-4ex}
        \caption{{IceClave performance (normalzied to ISC), as we vary the internal SSD bandwidth by using different number of channels. This figure refers to Figure~\ref{fig:bws-isc} in the revised paper.}}
        \label{fig:bws-isc-abs}
        \vspace{-2ex}
\end{figure}

\begin{figure}[!tph]
        \centering
        \includegraphics[width=\linewidth]{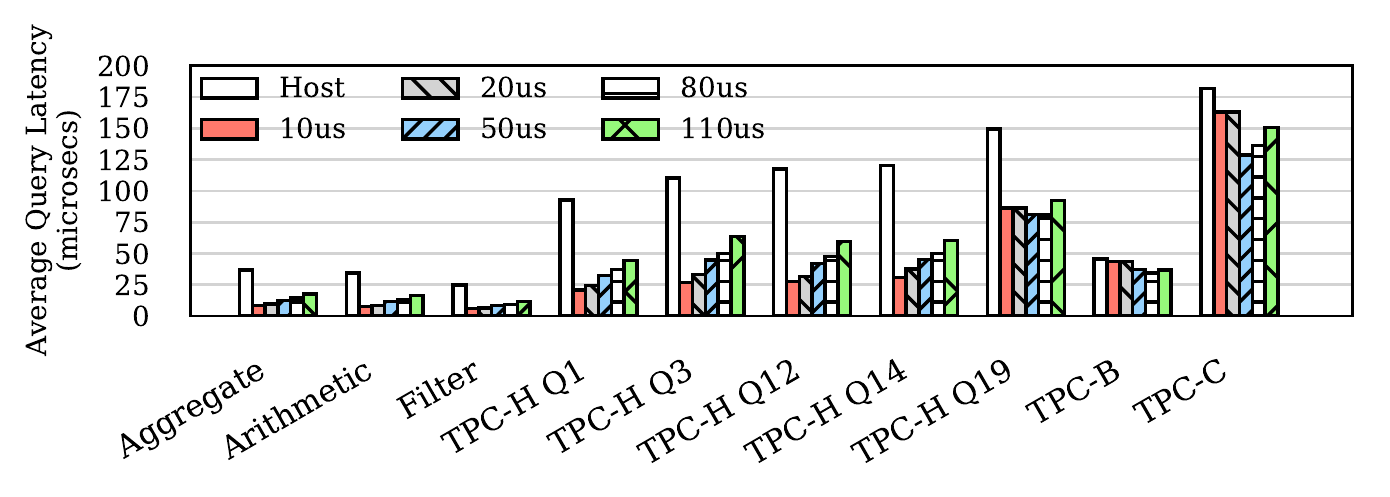}
        \vspace{-4ex}
        \caption{{Performance of IceClave as we vary the latency of accessing flash pages. This figure refers to Figure~\ref{fig:lat} in the revised paper.}}
        \label{fig:lat-abs}
        \vspace{-2ex}
\end{figure}

\begin{figure}[!tph]
        \centering
        \includegraphics[width=\linewidth]{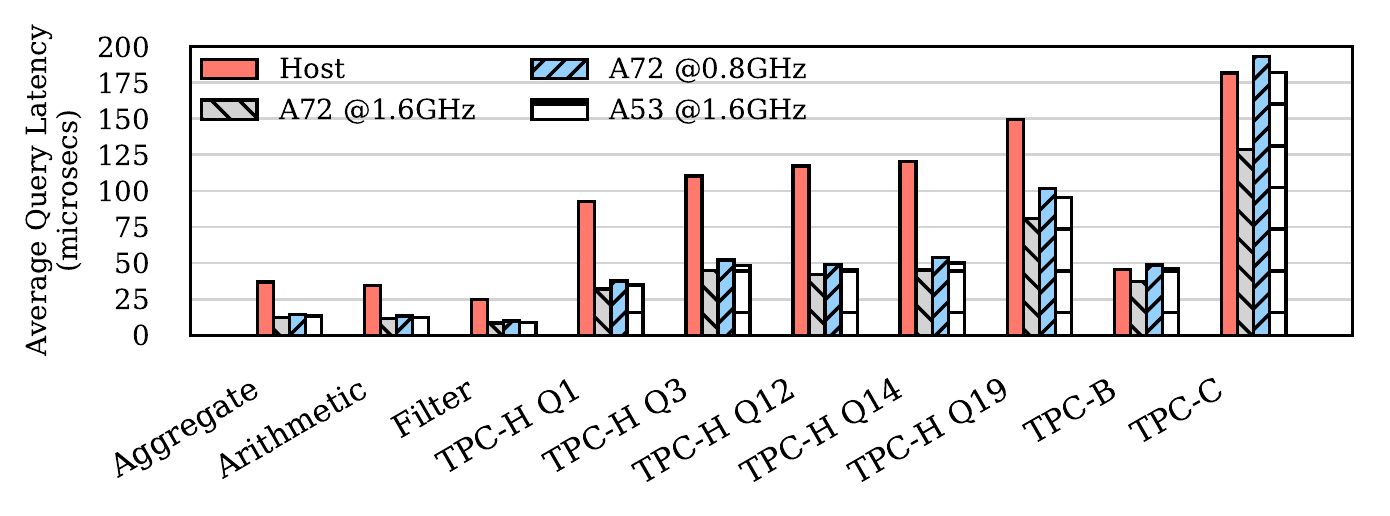}
        \vspace{-4ex}
        \caption{IceClave performance as we vary the in-storage computing capability. This figure refers to Figure~\ref{fig:core_ipc} in the revised paper.}
        }
        \label{fig:core_ipc-abs}
        \vspace{-3ex}
\end{figure}

\begin{figure}[!tph]
        \centering
        \includegraphics[width=\linewidth]{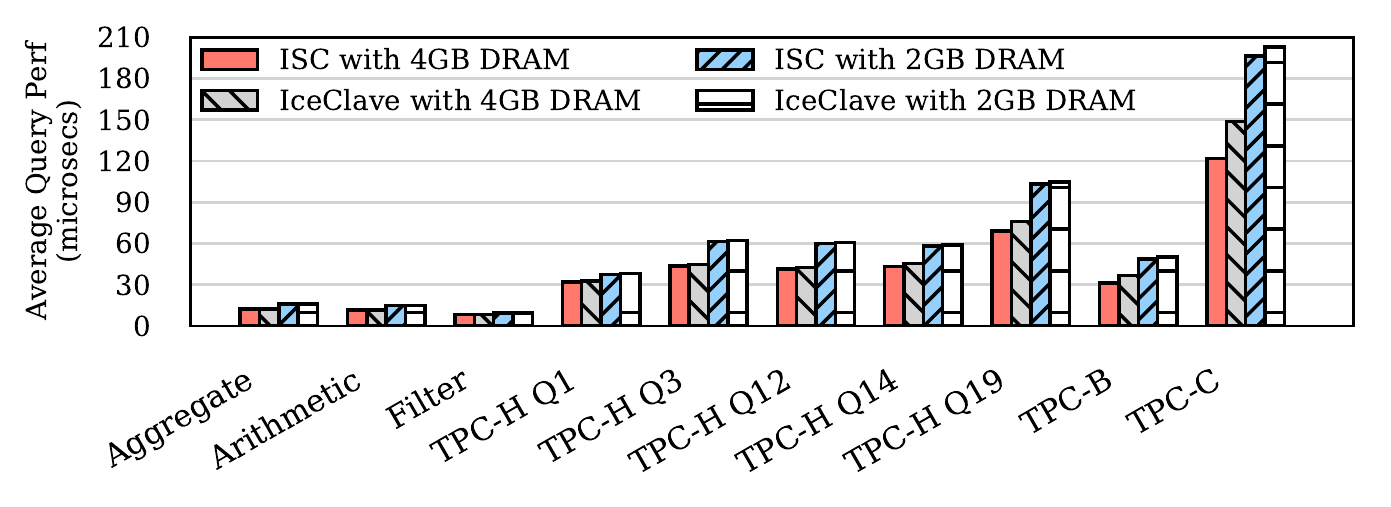}
        \vspace{-4ex}
        \caption{{IceClave performance with various SSD DRAM sizes. This figure refers to Figure~\ref{fig:dram-perf} in the revised paper.}
        }
        \label{fig:dram-perf-abs}
        \vspace{-3ex}
\end{figure}

\begin{figure}[!tph]
        \centering
        \includegraphics[width=\linewidth]{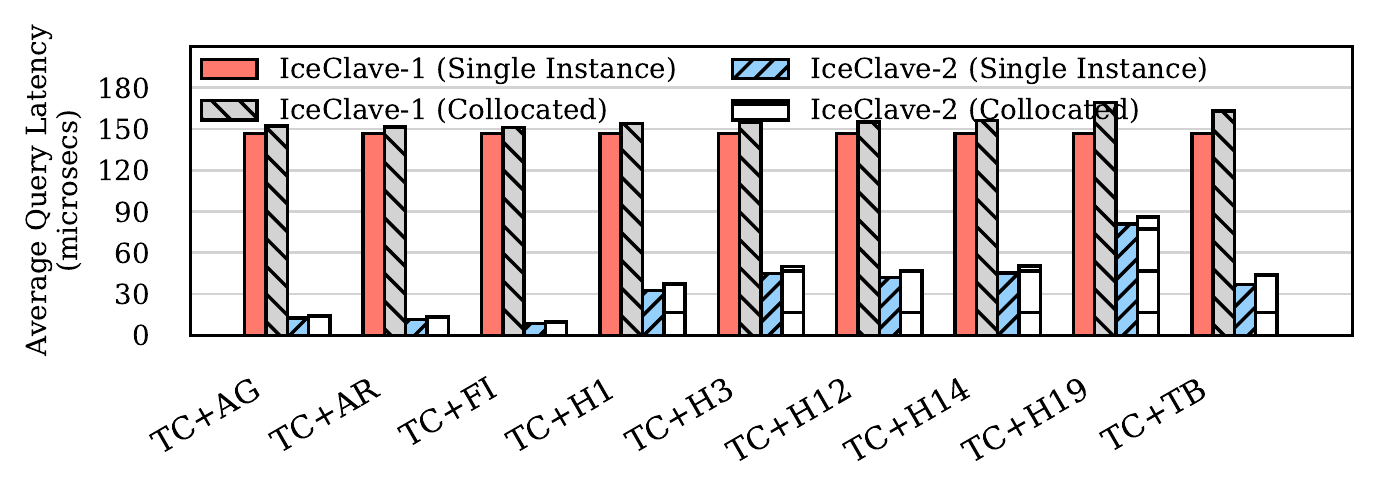}
        \vspace{-4ex}
        \caption{IceClave performance as we run two in-storage applications concurrently. 
        This figure refers to Figure~\ref{fig:twoclaves} in the revised paper.}
        \label{fig:twoclaves-abs}
        \vspace{-3ex}
\end{figure}

\begin{figure}[!tph]
        \centering
        \includegraphics[width=\linewidth]{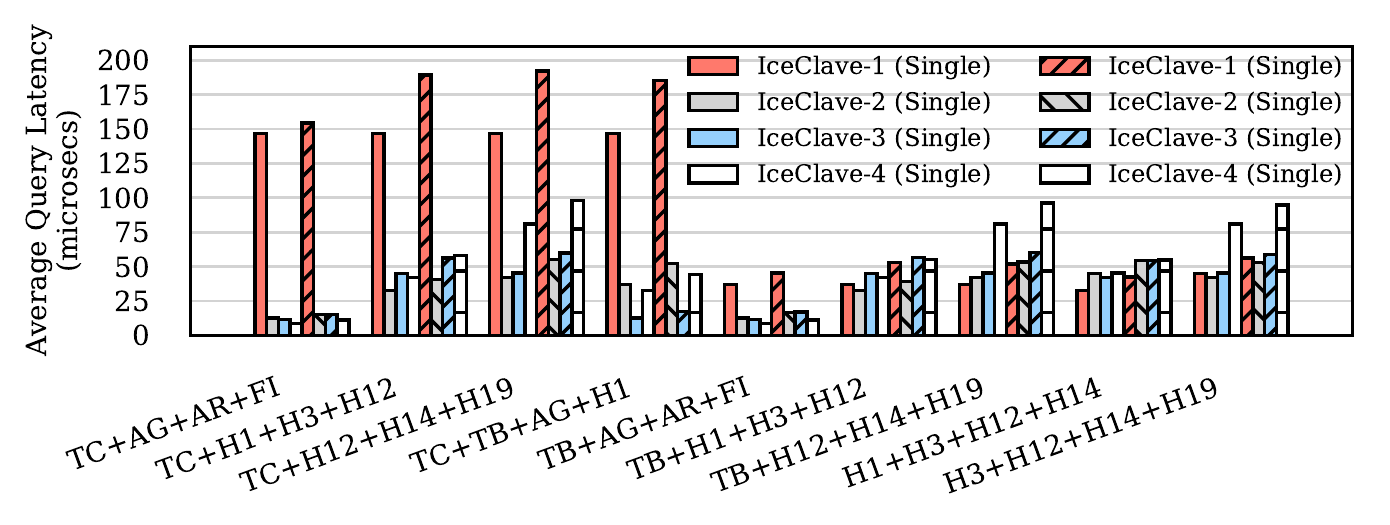}
        \vspace{-4ex}
        \caption{IceClave performance as we run four in-storage applications concurrently. 
	This figure refers to Figure~\ref{fig:fourclaves} in the revised paper.}
        \label{fig:fourclaves-abs}
        \vspace{-3ex}
\end{figure}
